# Supplementary material for: SAFER-Nav: Enhancing Safety for Visual Robot Navigation via Segmentation-Aware Fine-Tuning
Source: arXiv:2606.11636 source file (2026-09-18)
Supplement: Supplementary file 1 [file appendix.tex]

\appendix
\section*{\Large{Appendix}}

\section{Experimental Details}

We run experiments on three mobile platforms: RoboMaster S1, TurtleBot4, and LocoBot. Figure \ref{fig:robots} shows the actual hardware used in our experiments.

\begin{figure}[h]
    \centering

    \begin{subfigure}[t]{0.28\linewidth}
        \centering
        \includegraphics[width=\linewidth]{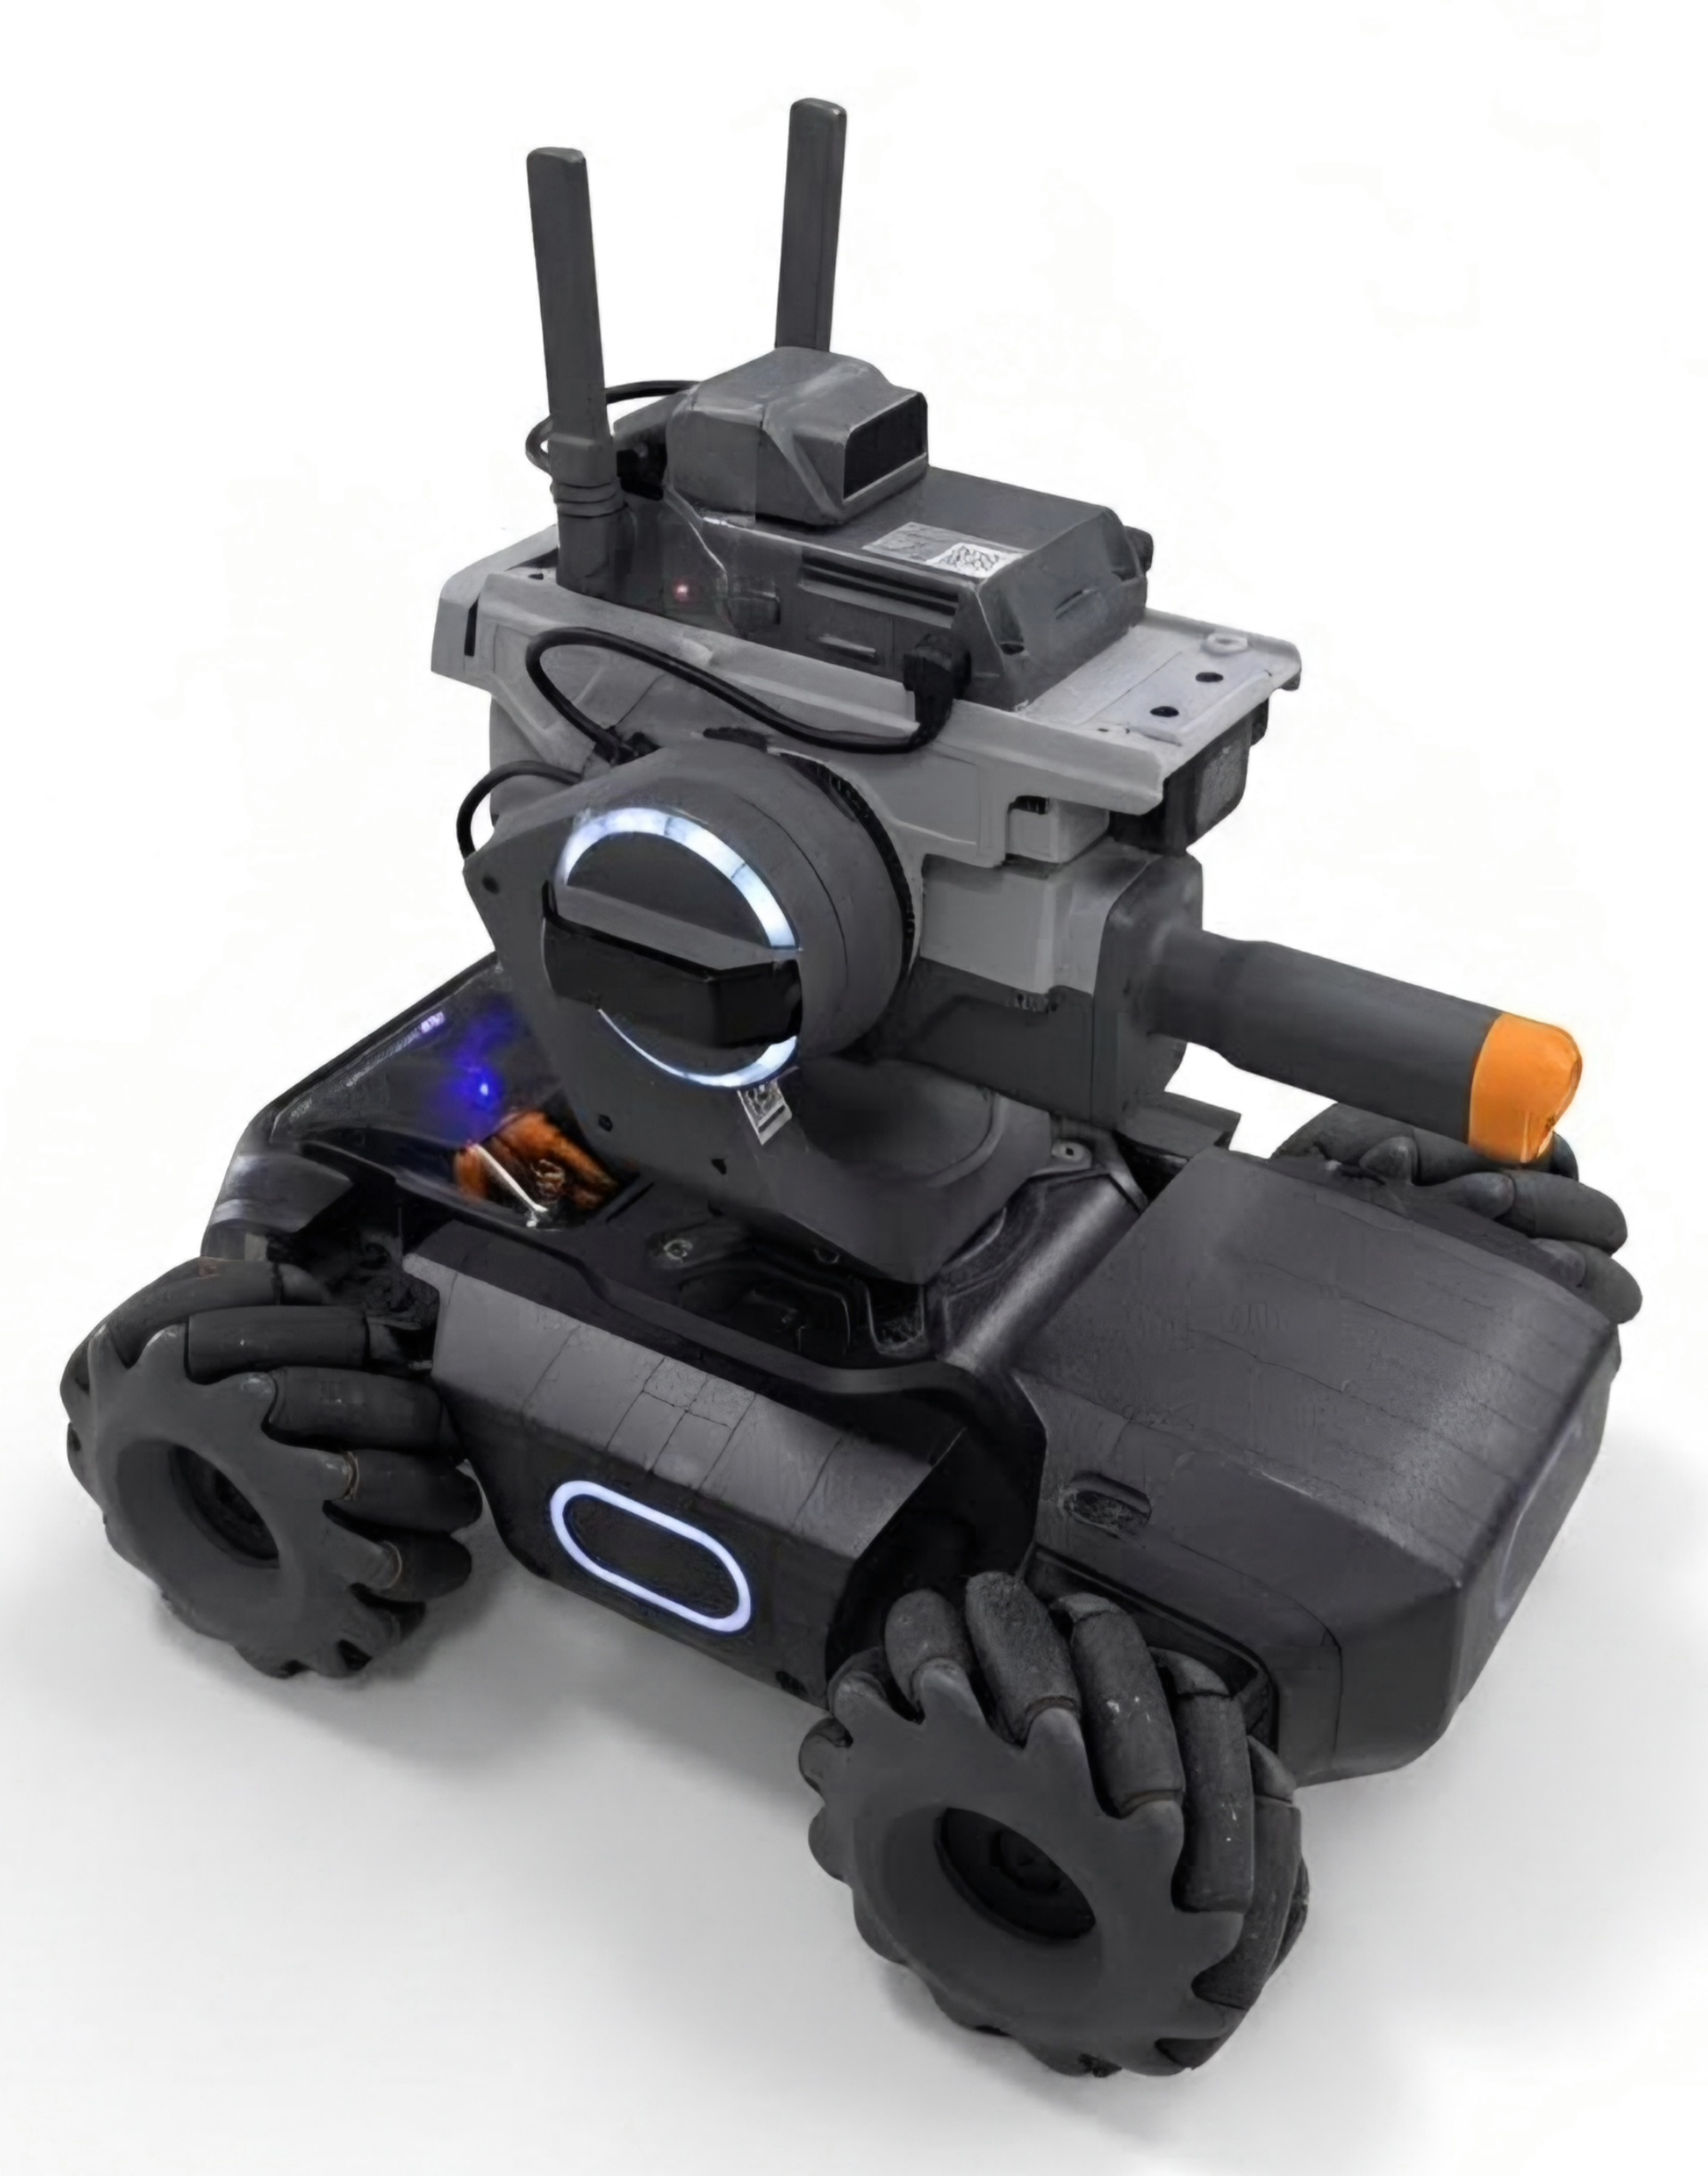}
        \caption{}
    \end{subfigure}
    \hfill
    \begin{subfigure}[t]{0.28\linewidth}
        \centering
        \includegraphics[width=\linewidth]{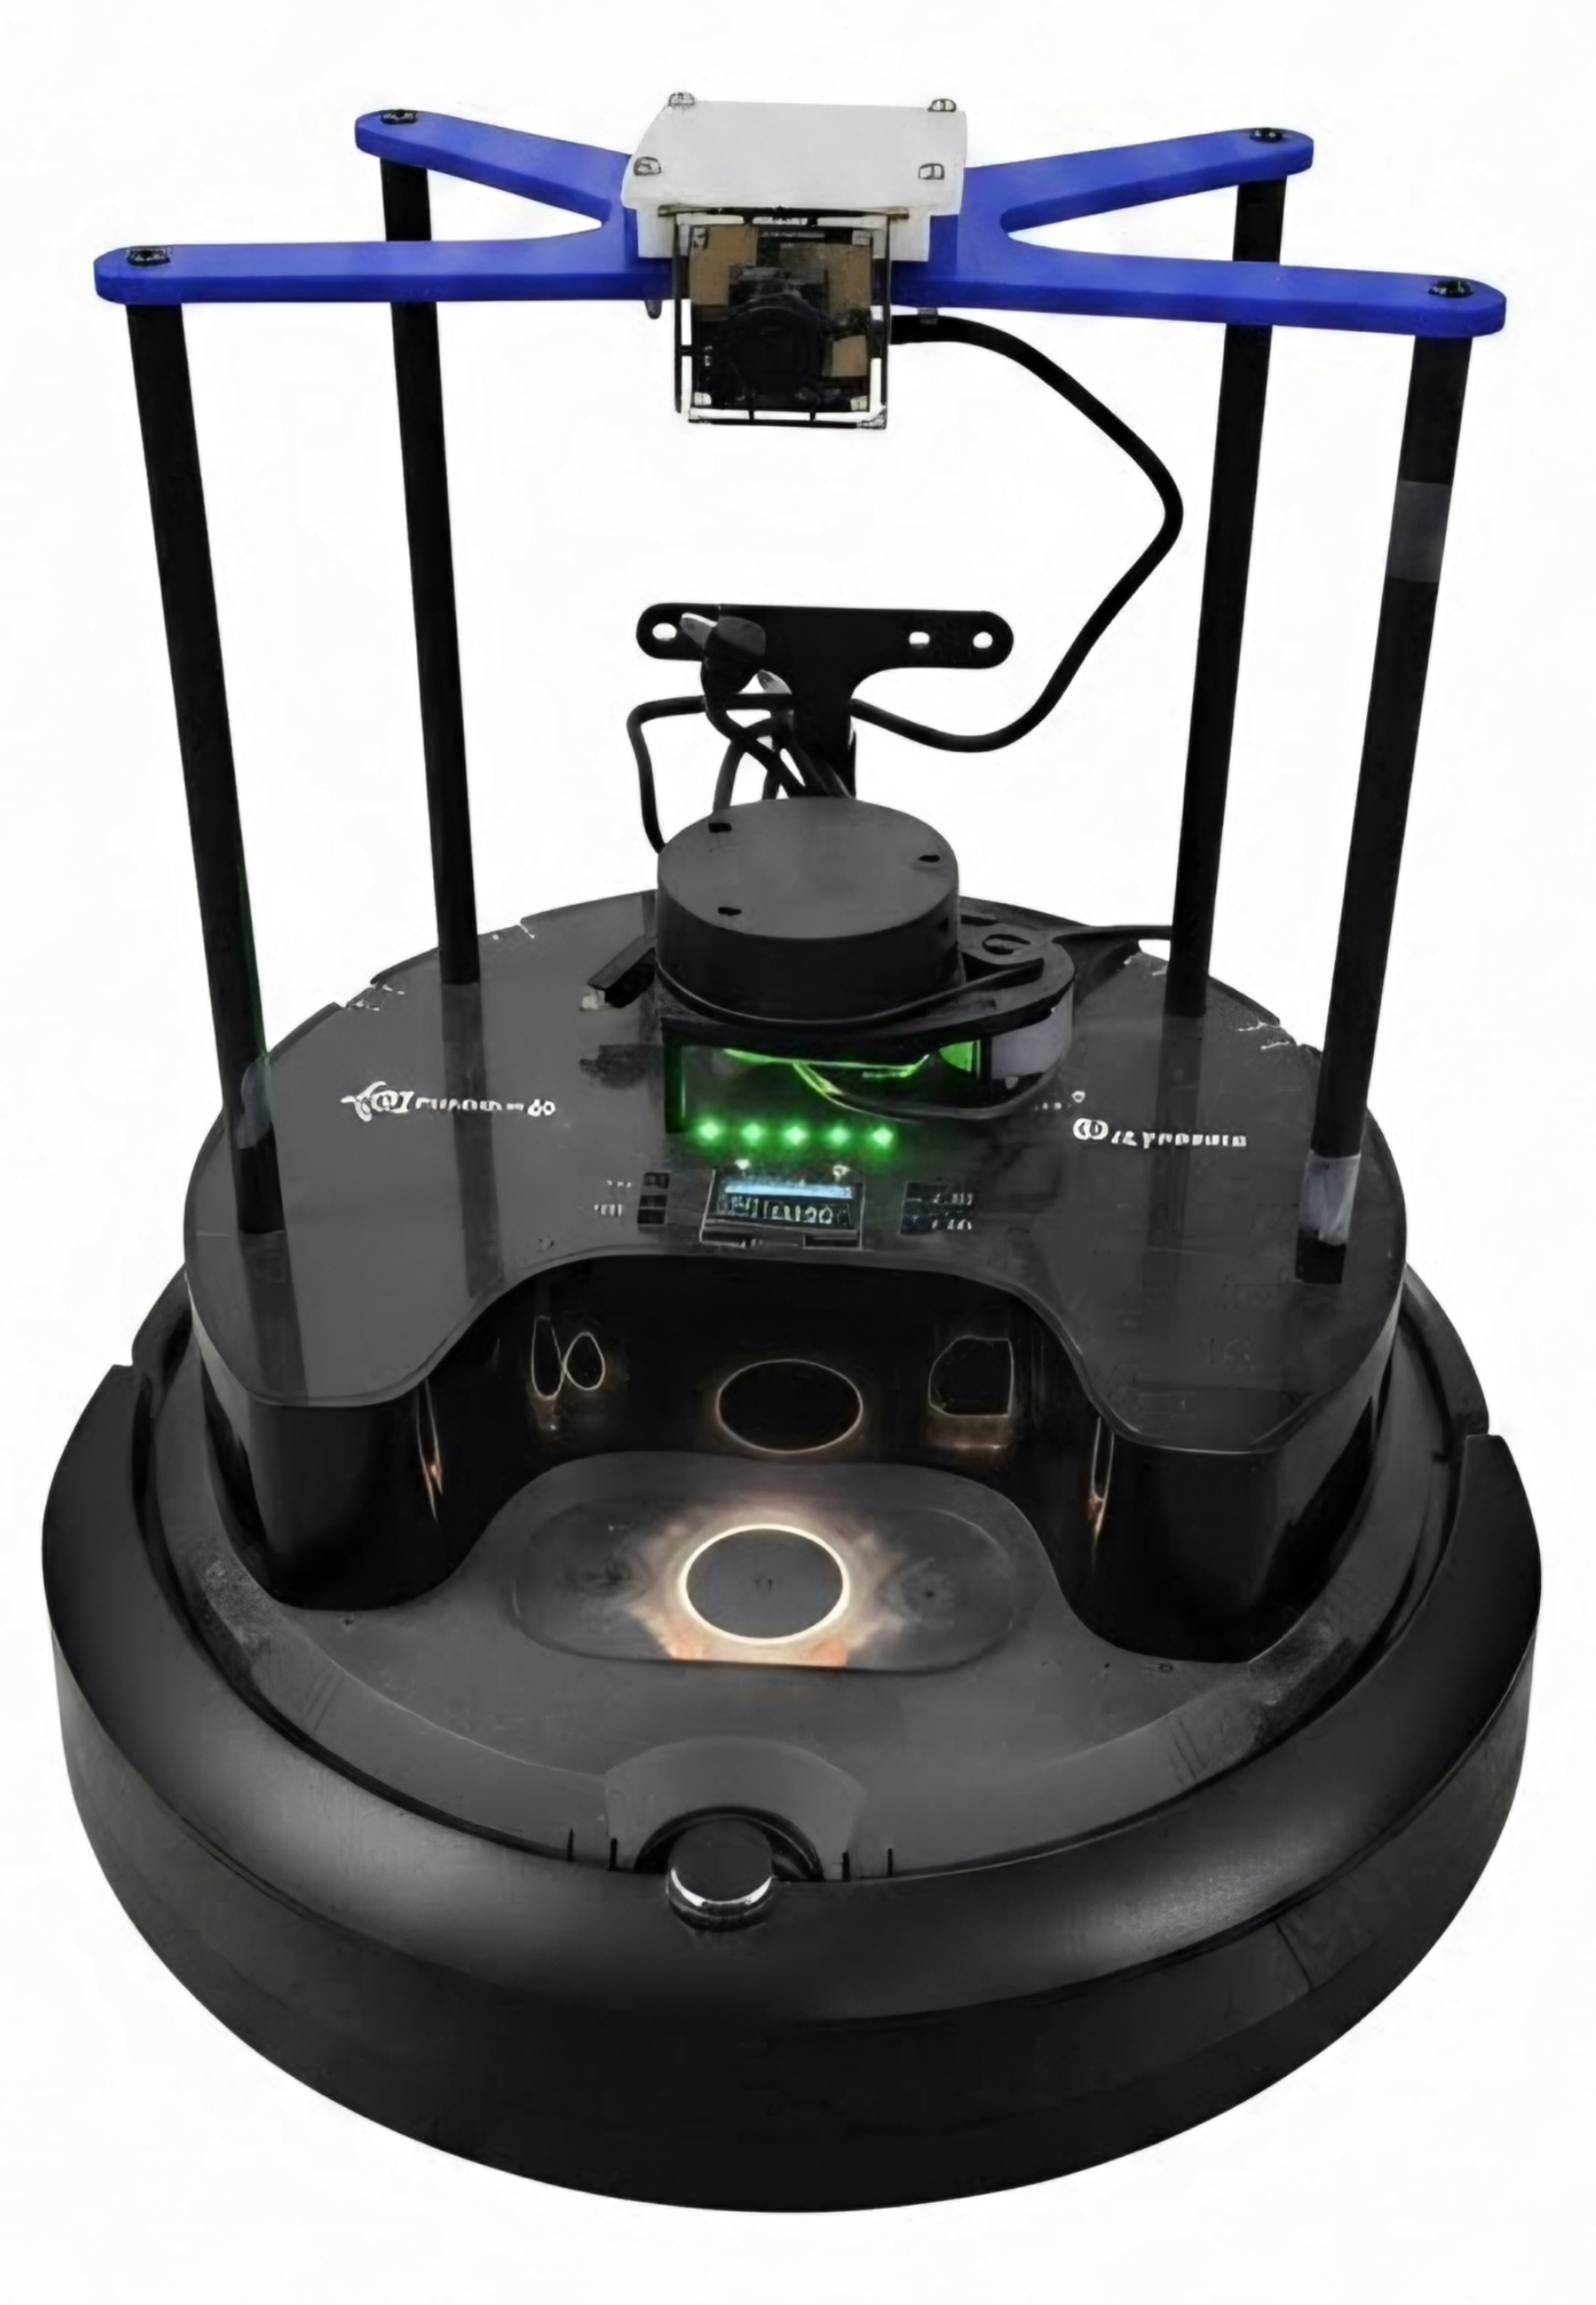}
        \caption{}
    \end{subfigure}
    \hfill
    \begin{subfigure}[t]{0.28\linewidth}
        \centering
        \includegraphics[width=\linewidth]{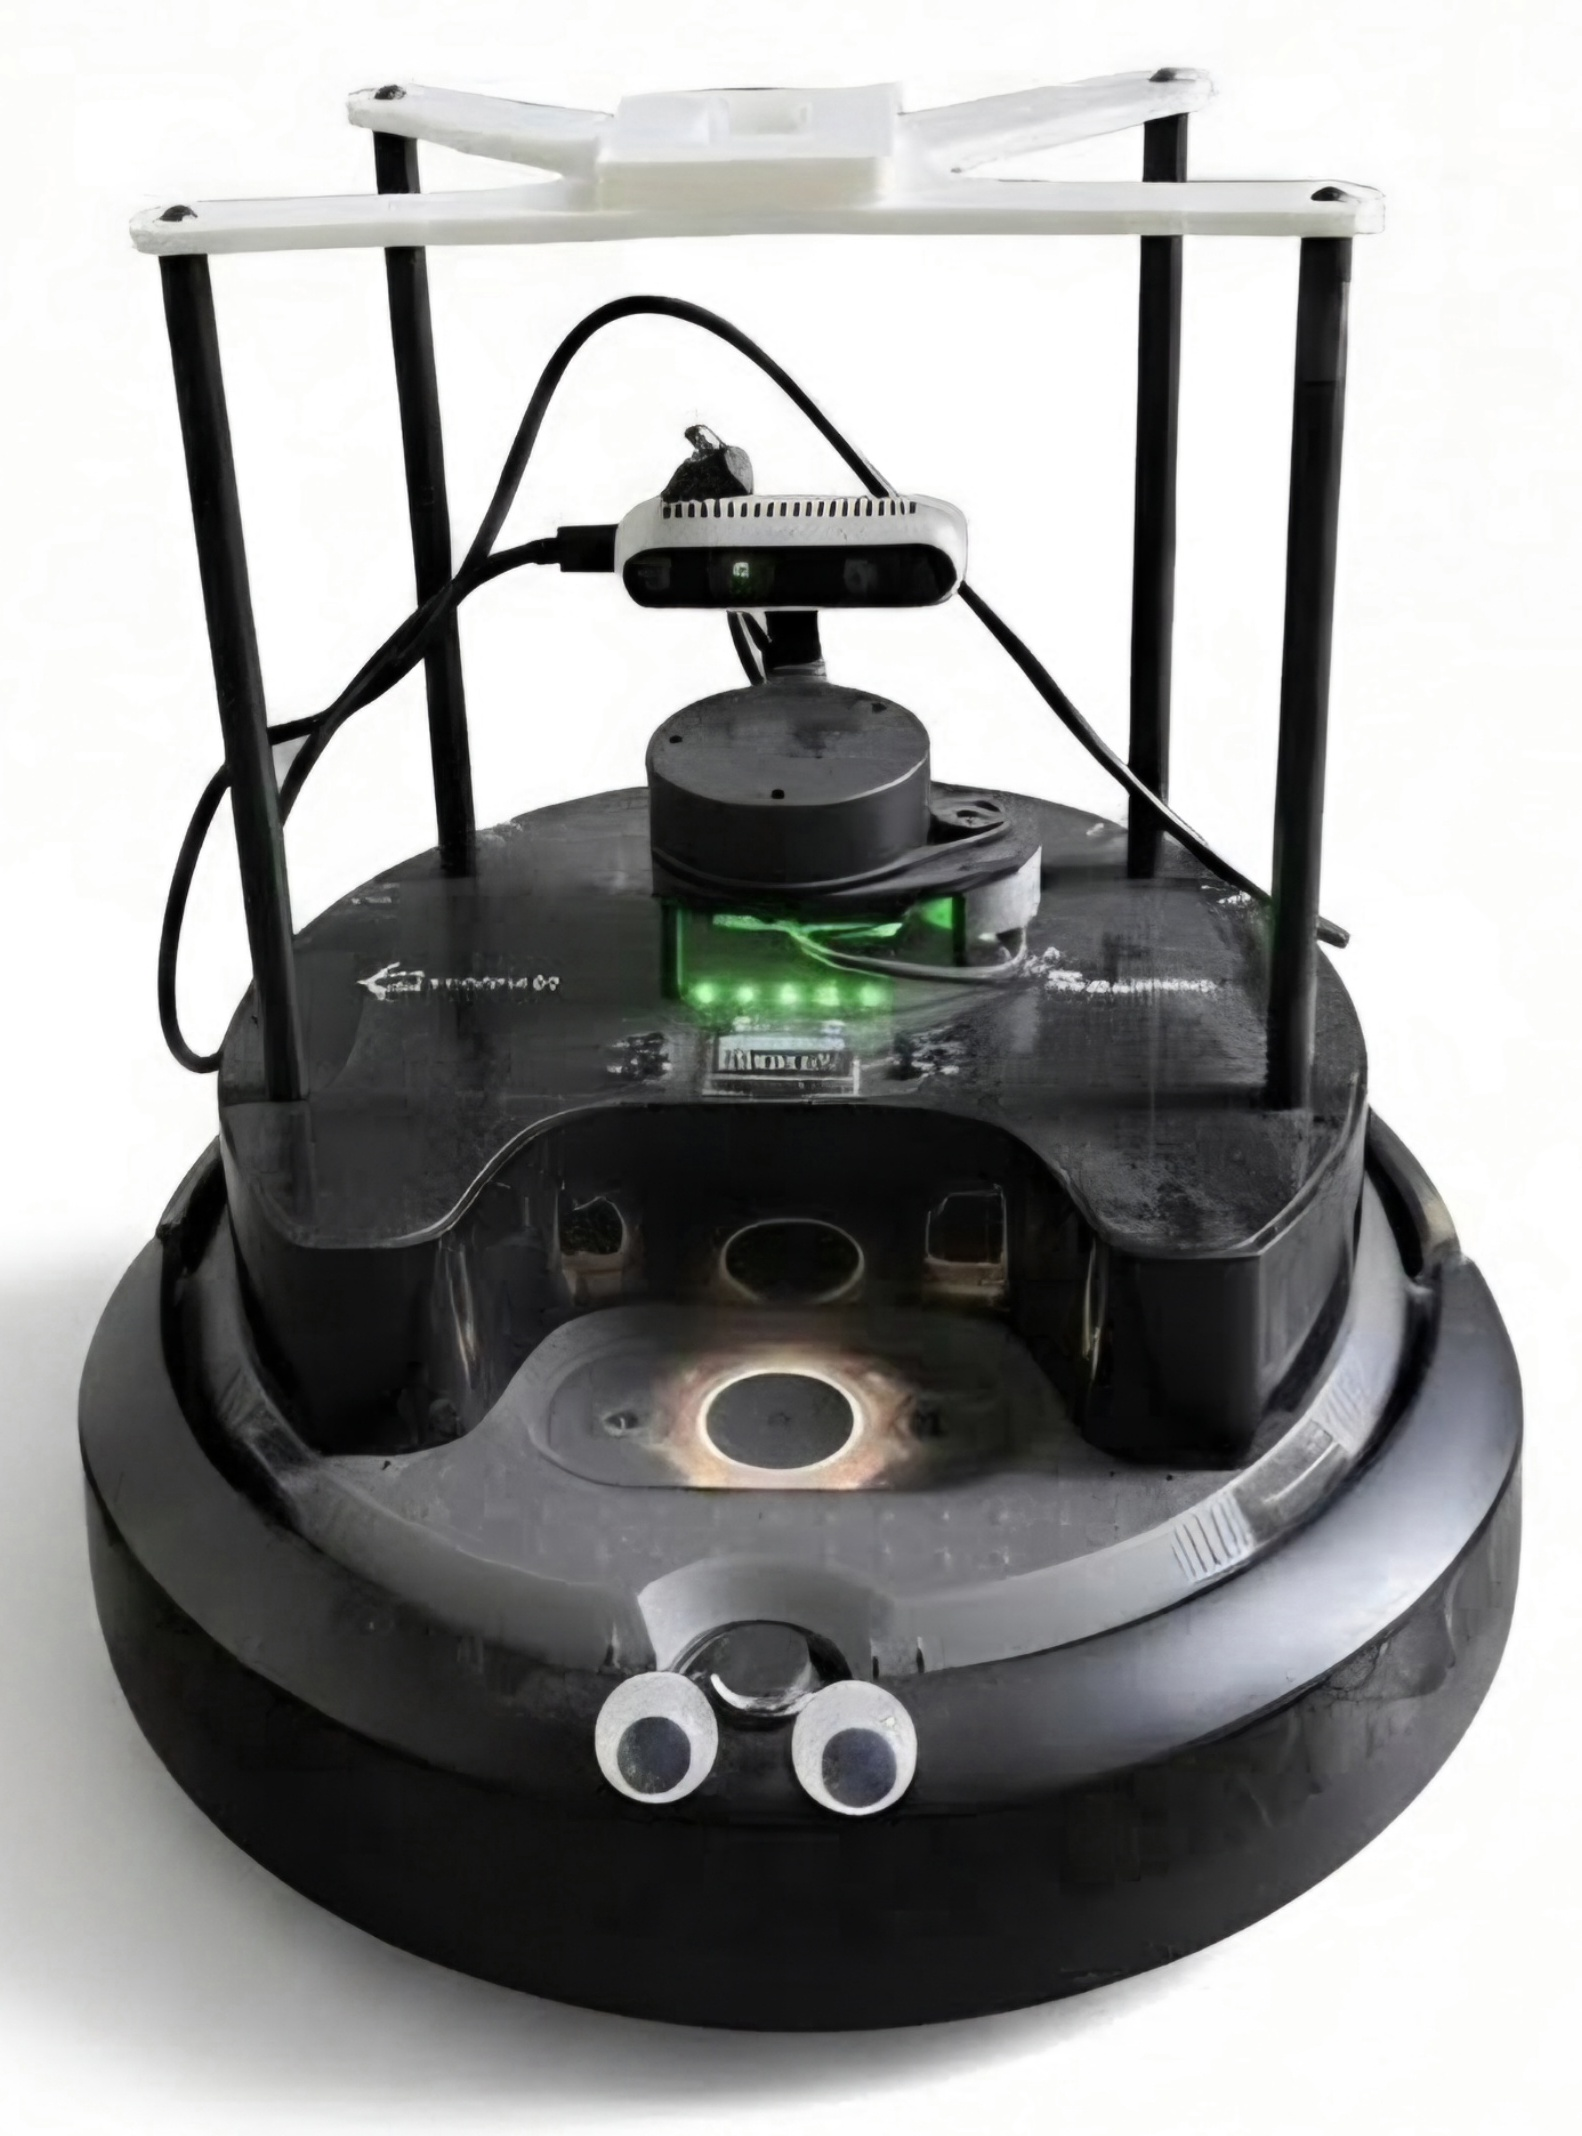}
        \caption{}
    \end{subfigure}

    \caption{Mobile robot platforms used for evaluation. Each robot was equipped with a monocular RGB camera.}
    \label{fig:robots}
\end{figure}

A note for LoCoBot. Although the original LoCoBot is built on a TurtleBot2 base, we implement our LoCoBot using a TurtleBot4 as TurtleBot2 has been discontinued. Nevertheless, two models are both differential drive type with very similar wheelbase width, wheel diameter, and etc. A custom 3D-printed camera mount is designed to match the fisheye camera position.

\begin{table}[h]
\centering
\caption{Robot-specific camera and platform parameters.}
\label{tab:robot_specs}
\begin{tabular}{lccc}
\toprule
\textbf{Specification} & \textbf{LoCoBot} & \textbf{TurtleBot4} & \textbf{RoboMaster S1} \\
\midrule
Published Image Resolution (pixels)       & $320 \times 240$ & $320 \times 200$ & $640 \times 360$ \\
Robot Size ($L \times W \times H$, mm)    & $341 \times 339 \times 350$ & $341 \times 339 \times 351$ & $320 \times 240 \times 270$ \\
Camera Height (mm)                        & 340            & 245            & 240            \\
Camera X-offset (mm)                      & 10             & -60            & 70             \\
\bottomrule
\end{tabular}
\end{table}

\begin{itemize}
    \item Published Image Resolution: The resolution of the RGB images published by each camera over ROS 2.
    \item Robot size (L × W × H): Physical dimensions of each robot, measured in millimeters (mm).
    \item Camera Height: The vertical distance from the ground to the optical center of the camera.
    \item Camera X-offset: The horizontal distance (in mm) between the geometric center of robots and the camera.
    \item A positive value indicates a forward-facing offset (camera mounted ahead of center), while a negative value indicates a rear-facing offset.
\end{itemize} 
